# Supplementary material for: Emulating two qubits with a four-level transmon qudit for variational quantum algorithms
Source: arXiv:2303.04796 source file (2024-03-21)
Supplement: Supplementary file 1 [file supplementary.tex]

\documentclass[aps, onecolumn, floatfix, superscriptaddress, amsmath, amssymb, longbibliography ]{revtex4-2}
 \pdfoutput=1

\input{preamble.tex}

\begin{document}

\title{Supplementary Materials for ``Emulating two qubits with a four-level  \\ transmon qudit for variational quantum algorithms''}

%\input{authors.tex}
%\date{\today}

\maketitle

%\begin{widetext}
\input{appendix}
%\end{widetext}
\bibliography{refnc}% Produces the bibliography via BibTeX.

\end{document}
